# Supplementary material for: Strong coupling electron-photon dynamics: a real-time investigation of energy redistribution in molecular polaritons
Source: arXiv:2404.09762 source file (2024-04-15)
Supplement: Supplementary file 1 [file SI.pdf]

# Supplemental Information: Strong coupling electron-photon dynamics: a real-time investigation of energy redistribution in molecular polaritons

Matteo Castagnola,[†] Marcus T. Lexander,[†] Enrico Ronca,[*,‡] and Henrik Koch[*,†]

†*Department of Chemistry, Norwegian University of Science and Technology, 7491 Trondheim, Norway*

‡*Dipartimento di Chimica, Biologia e Biotecnologie, Università degli Studi di Perugia, Via Elce di Sotto, 8,06123, Perugia, Italy*

E-mail: enrico.ronca@unipg.it; henrik.koch@ntnu.no

# Contents

**S1 Computational details** **S2**

**S2 Implementation of the RT-QED-CC equations** **S3**

**S3 Additional results** **S5**

S3.1 Additional $(H_2)_2$ data . . . . . . . . . . . . . . . . . . . . . . . . . . . . . . . . . S5

S3.2 Additional succinic semialdehyde $C_4H_6O_3$ data . . . . . . . . . . . . . . . . . . S10

**S4 Real-time QED-CC equations** **S12**

**S5 Molecular geometries** **S14**

**References** **S17**

# S1 Computational details

All the calculations have been performed with a private branch of the $e^{\mathcal{T}}$ program.[1] Videos of the energy transfer dynamics and output files are available in a Zenodo repository `DOI: 10.5281/zenodo.10813660`

The $(H_2)_2$ system is described in the 6-31++g** basis set, with one $H_2$ oriented along the x axis and the other on the y axis. The molecular geometries are reported in section S5. The system is excited with an external pulse

$$\boldsymbol{E}(t) = \boldsymbol{\mathcal{E}}(t) \cos(\omega_e t + \phi) \tag{1}$$

with carrier frequency $\omega_e = 0.464\,408\,577$ a.u. (resonant to the first bright excitation of one $H_2$) and phase shift $\phi = 0$. The envelope function $\mathcal{E}(t)$ is a gaussian with maximum intensity $\boldsymbol{\mathcal{E}}_0 = 0.05$ a.u. and width 2.0 a.u., polarized along x. The equations are propagated for at least 2000 a.u. of time using a Runge-Kutta integrator with a time step of 0.005 a.u., and

the energies, the dipole moments, photon coordinate, amplitudes, multipliers, electric field, and density matrices are recorded every 0.25 a.u.. The densities are visualized on the xy plane by using the density matrices to construct a cube file on a grid of 0.1 Å spacing, and the ground state density was subtracted to the density of each snapshot to obtain the density displacement. The QED photon field is tuned to the $H_2$ excitation energy ($\omega = 0.464\,408\,577$ a.u.) and polarization along the xy bisector line $\boldsymbol{\epsilon} = (\frac{1}{\sqrt{2}}, \frac{1}{\sqrt{2}}, 0)$. The light-matter coupling strength is $\lambda = 0.01$ a.u. unless stated otherwise, and we consider a single photon mode. In this way, the photon field is coupled to both hydrogens, but the external pulse only excites one of them.

The succinic semialdehyde $C_4H_6O_3$ is studied in the 6-31g* basis set and oriented such that the carbon and oxygens of the acidic group lie in the xy plane (the aldehydic group is also *almost* lying in the same plane). The molecular geometry is reported in section S5 in Table S11. The system is excited with an external pulse as in Equation 1, but we used a sine-squared envelope function. The carrier angular frequency now is $\omega_e = 0.272\,216\,406\,0$ a.u. (resonant to the excitation II reported in the main text, mainly localized on the acid group) and phase shift $\phi = 0$, with a peak strength of $\boldsymbol{\mathcal{E}}_0 = 0.001$ a.u., width 45.0 a.u., and polarized along x. The equations are propagated for at least 250 a.u. of time using a Runge-Kutta integrator with a time step of 0.005 a.u., and the energies, the dipole moments, photon coordinate, amplitudes, multipliers, electric field, and density matrices are recorded every 0.25 a.u.. The QED photon field is tuned to the excitation III reported in the main text (mainly localized on the aldehyde) $\omega = 0.286\,743\,5$ a.u. with light-matter coupling strength $\lambda = 0.05$ a.u. and polarized along $\boldsymbol{\epsilon} = (\frac{1}{\sqrt{2}}, \frac{1}{\sqrt{2}}, 0)$.

# S2 Implementation of the RT-QED-CC equations

The RT-QED-CCSD-1 equations have been implemented in a development version of the $e^{\mathcal{T}}$ program.[1] For debugging purposes, we cannot resort to a real-time QED-FCI implementation

since, even for two-electron systems like $H_2$, $HHe^+$, and He, the photon degrees of freedom are modeled differently. QED-FCI relies on a CI truncation of the photon Fock space, while the exponential of the photon excitation in QED-CC $e^{\gamma b^\dagger}$ is similar to a photon coherent state, having components in the whole photon Fock space. The QED-FCI and QED-CC results are thus different also for two-electron systems. We must then find a different path to prove the correctness of our implementation.

First, our implementation for quenched light-matter coupling strength $\lambda = 0$ recovers the RT-CCSD dynamics. Although necessary, this is clearly not enough. Therefore, we follow the ideas presented in Ref.[2] and implement a propagation of the RT-QED-CCSD-1 equations in imaginary time, that is, with the substitution $t \to -it$. An eigenstate of energy $E'$ of the Hamiltonian evolves in time, only changing its global phase $e^{-iE't} \to e^{-E't}$, and therefore, the excited states will show a faster exponential decay than the ground state.[3] Moreover, the CC parametrization always ensures an intermediate normalization

$$\langle HF|e^T|HF\rangle = 1, \tag{2}$$

and thus, no renormalization is necessary. Therefore, regardless of the initial amplitudes, after enough time has passed on the imaginary time propagation simulation, the state will decay onto the QED-CC ground state. This is readily verified with our implementation of the RT-QED-CCSD-1, and in Figure S1 we report the energy of the imaginary time propagation for an $H_2O$ molecule in an optical cavity of frequency $\omega = 0.371\,048$ a.u. with light-matter coupling strength $\lambda = 0.1$ a.u. and polarization along the $C_2$ axis of the molecule, using the 6-31g* basis set. The initial state of the simulation is the QED-HF state, corresponding to the cluster operator $T = 0$ and Lagrange multipliers $\bar{t}_{\mu n} = 0$, which is then propagated for 30 a.u. of time with a time step of 0.01 a.u. using a Runge-Kutta integrator. The energy of the system (panel B in Figure S1) quickly converges to the QED-CCSD ground state energy, and so do the amplitudes, the Lagrange multipliers, and molecular properties such as the permanent

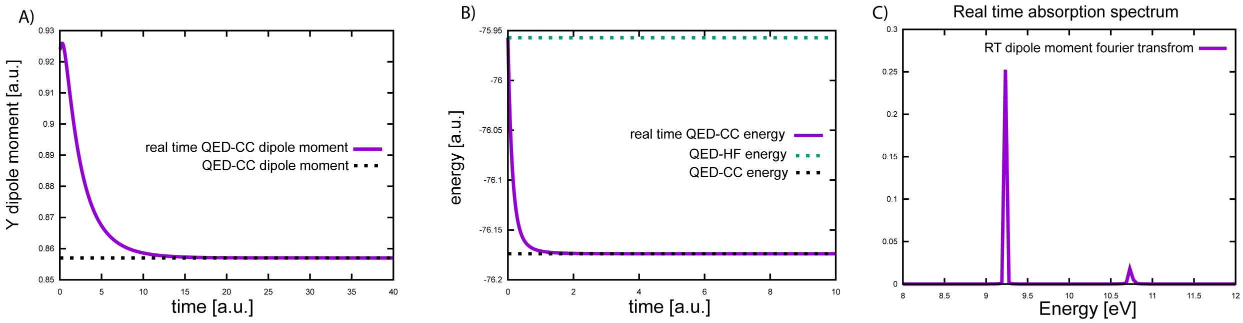


Figure S1: A) y component of the dipole moment of a 6-31g* water molecule starting from the QED-HF state and propagating over imaginary time $t \to it$. The dipole moment quickly converges to the ground state QED-CCSD expectation value. B) Energy of a 6-31g* water molecule starting from the QED-HF state and propagating over imaginary time $t \to it$. The energy quickly converges to the QED-CCSD ground state energy. C) Absorption spectrum of a 6-31g* water molecule after excitation with a short electric pulse computed via fast Fourier transform of the propagation of the y component of the dipole moment. The excitation energies and the intensities are consistent with the EOM-QED-CCSD-1 calculations.

dipole moment (panel A in Figure S1) and the photon coordinate. Finally, performing a simulation in real-time (no imaginary time propagation) following the excitation of the system with an electric pulse (central time 1.0 a.u., carrier angular frequency 0.371 048 a.u., peak intensity 0.05 a.u., width 0.2 a.u., polarized along the $C_2$ axis of water), we can compute the absorption spectrum by a fast Fourier transform of the dipole moment. The spectrum is reported in panel C of Figure S1 after propagating the system for 4000.0 a.u., and the computed peaks and intensities agree with the EOM-QED-CCSD-1 simulation.

# S3 Additional results

In this section, we include additional results for the systems discussed in the main text.

## S3.1 Additional $(H_2)_2$ data

In Figure S2, we report the dipole moments after exciting the $(H_2)_2$ system with an external pulse. The left panels refer to the geometry in Table S9 while the right panels refer to the geometry in Table S10, with light-matter coupling strengths $\lambda = 0.01$ a.u. and 0.005 a.u. (top

to bottom respectively). The time scale of the photon-mediated energy transfer is reduced by a factor of 2 in the simulations with $\lambda = 0.005\,\text{a.u.}$ compared to $\lambda = 0.01\,\text{a.u.}$. This result is reasonable as the photon-mediated time scales are determined by the Rabi splittings, which are almost linear in $\lambda$. Notice, however, that the introduction of intermolecular interactions effectively detunes the cavity from the molecular excitations, so the behavior is not expected to be perfectly linear. The dipole self-energy, although small, generates a similar detuning effect. Nevertheless, in about twice the time compared to $\lambda = 0.01\,\text{a.u.}$, the same amount of

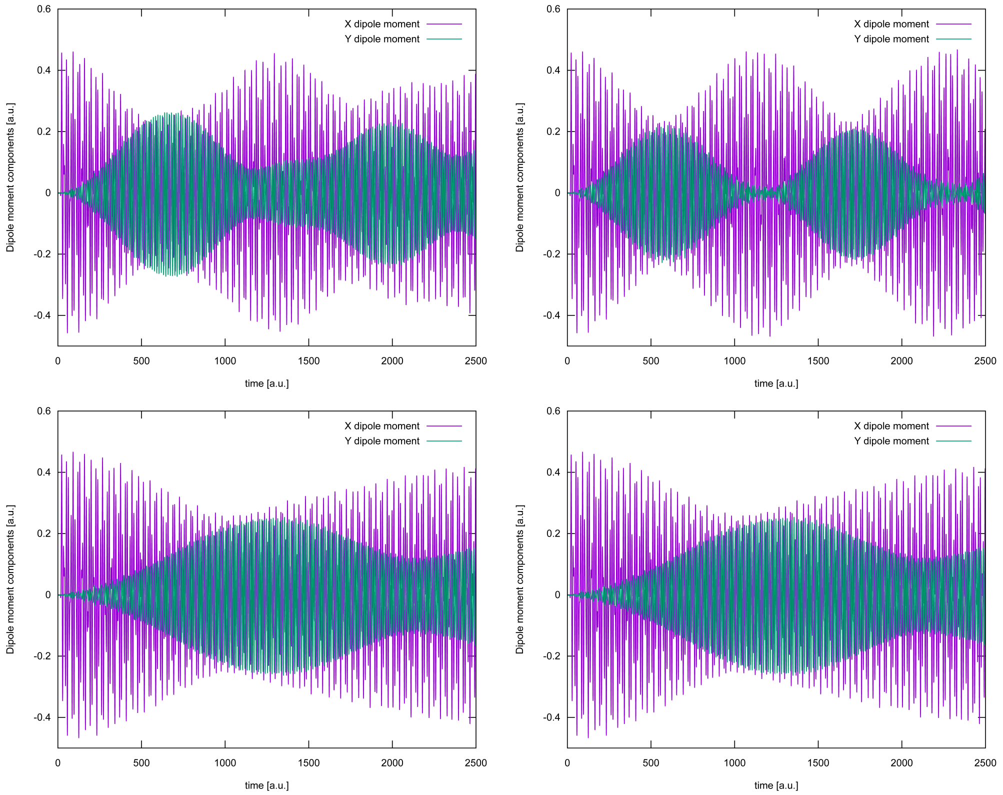


Figure S2: Dipole moments after exciting the $(H_2)_2$ system with an external pulse. The left panels refer to the geometry in Table S9 while the right panels refer to the geometry in Table S10. In the upper panels, the light-matter coupling strength is set to 0.01 a.u. as in the figures in the main text, while the lower panels are computed using $\lambda = 0.005\,\text{a.u.}$ and therefore have different time scales.

energy transfer can be achieved (if decoherence processes are suppressed). On the other hand, the electronic energy transfer (Förster and Dexter) is almost unaffected by any modification of the properties of the optic device (the dipole self-energy here only introduces a tiny shift

of the molecular energies). The same conclusions can be drawn from the photon coordinate, plotted in Figure S3 for the $(H_2)_2$ system of Table S9. Notice that no energy transfer occurs

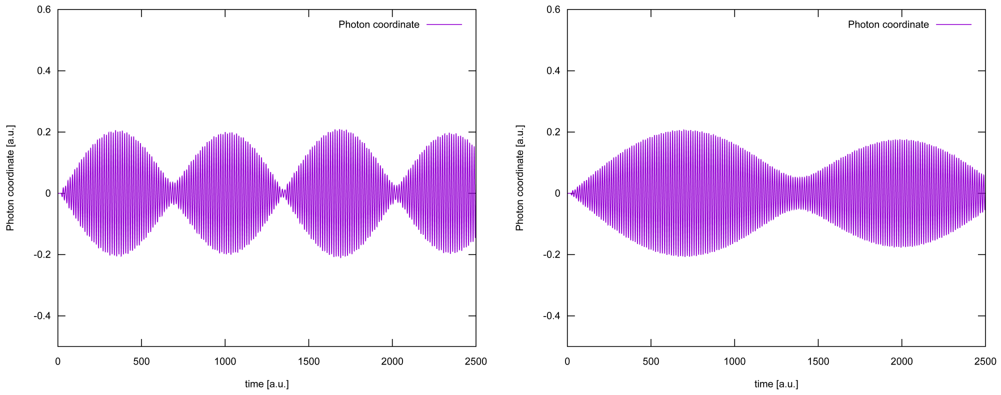


Figure S3: Photon coordinate after exciting the $(H_2)_2$ system with geometry in Table S9. The left panel and right panels are computed using $\lambda = 0.01$ a.u. and 0.005 a.u. respectively, and therefore have different time scales.

without the mediation of the cavity photon, as seen from the out-of-cavity simulation in

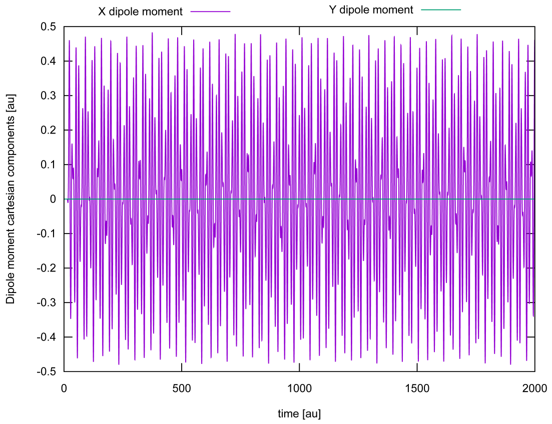


Figure S4: Dipole moment after exciting the $(H_2)_2$ system with geometry in Table S9 outside the cavity (no QED).

It is also interesting to investigate how these quantities would change by increasing the number of replicas in the simulation $((H_2)_2)_N$ while rescaling the coupling strength by $1/\sqrt{N}$, thus keeping the Rabi splitting constant. In Figure S5, we report the computed dipole moments and photon coordinates, and in Table S5 we report the energies of the system before and after the interaction with the pulse for $N = 2$ and 3. All the systems are subject

to the same electric pulse described in section S1. The energy gained from the interaction

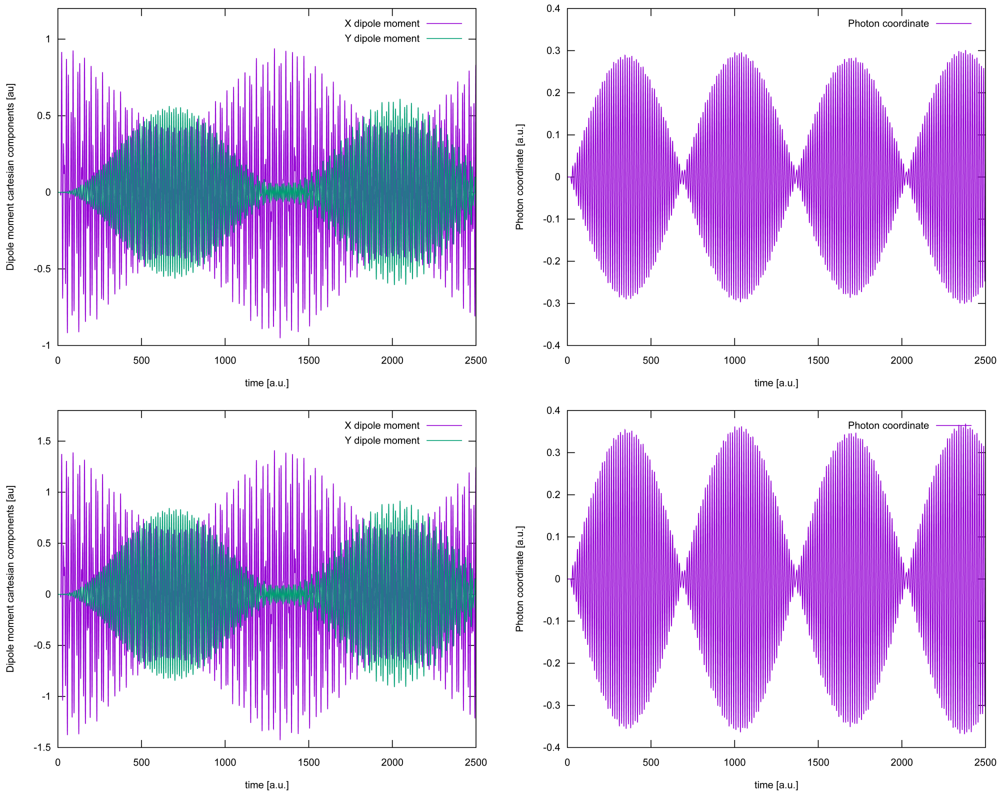


Figure S5: Dipole moment and photon coordinate for two (upper panels) and three (lower panels) identical $(H_2)_2$ systems (placed at 300 Å distance and with geometry in Table S7) after excitation with the same pulse as Figure S2. The coupling strength has been rescaled by a factor of $1/\sqrt{2}$ and $1/\sqrt{3}$ to $\lambda = 0.007\,071\,067\,8$ a.u. and $0.005\,773\,502\,6$ a.u. to keep the Rabi splitting constant.

with the external pulse increases linearly with the number of replicas $N$, as expected since the energy absorption depends on the number of interacting molecules (the size-intensivity and extensivity of the CC parametrization are a fundamental aspect of the theory). This is also reflected in the linear $N$ scaling of the oscillation amplitude of the dipole moment in Figure S5 (see the main text for the results of a single $(H_2)_2$). In addition, the time scales are the same in these simulations, as expected, since they show the same Rabi splitting. The time scales, therefore, are only determined by the *collective* coupling strength $\lambda\sqrt{N}$. On the other hand, the amplitudes of the photonic properties scale as the square root $\sqrt{N}$ of the number of replicas, which suggests that a relevant amount of energy is stored in the dark

states. Therefore, photon and matter quantities have a different scaling with the number of replicas, when all the systems are subject to the same external pulse. The same conclusions are drawn for the $(H_2)_2$ system with slightly different bond length (geometry in Table S8), as reported in Figure S6

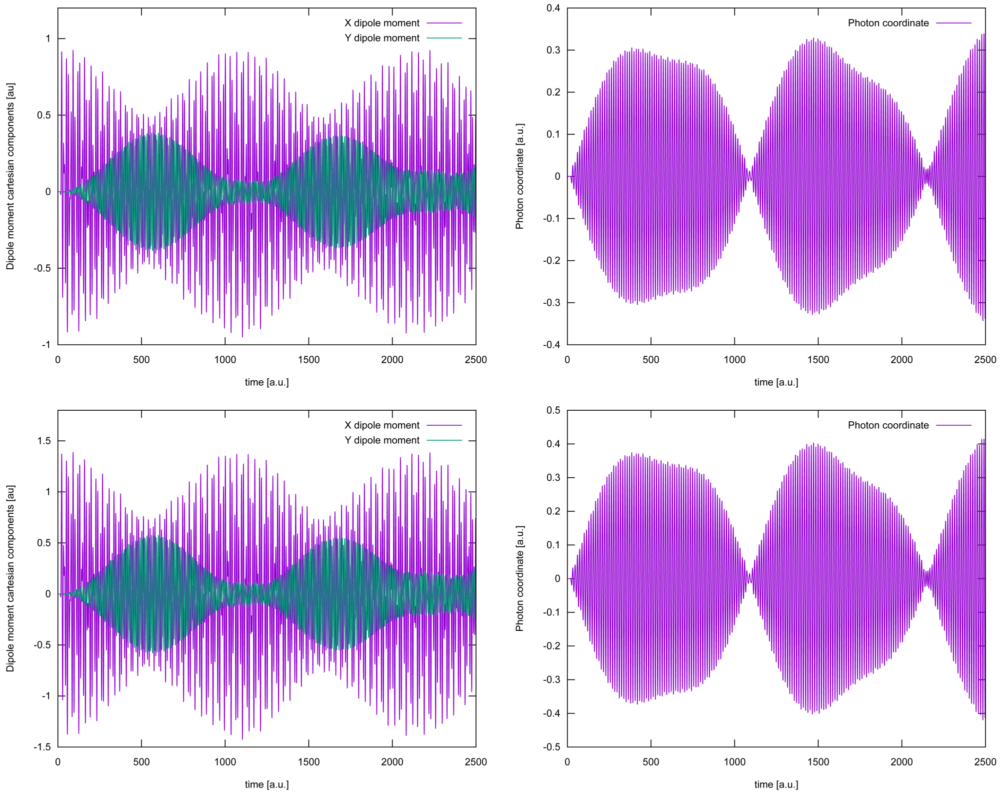


Figure S6: Dipole moment and photon coordinate for two (upper panels) and three (lower panels) identical $(H_2)_2$ systems (placed at 300 Å distance and with geometry in Table S8) after excitation with the same pulse as Figure S2. The coupling strength has been rescaled by a factor of $1/\sqrt{2}$ and $1/\sqrt{3}$ to $\lambda = 0.007\,071\,067\,8$ a.u. and $0.005\,773\,502\,6$ a.u. to keep the Rabi splitting constant.

In Table S1, we report the energy of the $(H_2)_2$ system of Table S7 (identical perpendicular hydrogens, $D = 50$ Å) before and after the interaction with the external pulse.

**Table S1: Energy of the $(H_2)_2$ system of Table S7 before and after before and after the interaction with the external pulse. Computational details are reported in section S1**

| Energy [a.u.] | Initial | Pulse 1 |
|---|---|---|
| QED simulation | -2.32991 | -2.31173 |

In Table S2, we report the energy of the $(H_2)_2$ system of Table S8 (perpendicular hydrogens of bond lengths 0.76 Å and 0.78 Å, $D = 50$ Å) before and after the interaction with the external pulse.

**Table S2: Energy of the $(H_2)_2$ system of Table S8 before and after before and after the interaction with the external pulse. Computational details are reported in section S1**

| Energy [a.u.] | Initial | Pulse 1 |
|---|---|---|
| QED simulation | -2.32914 | -2.31096 |

In Table S3, we report the energy of the ( $H_2)_2$ system of Table S9 (identical perpendicular hydrogens, $D = 5$ Å) before and after the interaction with the external pulse.

**Table S3: Energy of the $(H_2)_2$ system of Table S9 before and after before and after the interaction with the external pulse. Computational details are reported in section S1**

| Energy [a.u.] | Initial | Pulse 1 |
|---|---|---|
| QED simulation | -2.32993 | -2.31176 |

In Table S4, we report the energy of the $(H_2)_2$ system of Table S10 (perpendicular hydrogens of bond lengths 0.76 Å and 0.78 Å, $D = 5$ Å) before and after the interaction with the external pulse.

**Table S4: Energy of the $(H_2)_2$ system of Table S10 before and after before and after the interaction with the external pulse. Computational details are reported in section S1**

| Energy [a.u.] | Initial | Pulse 1 |
|---|---|---|
| QED simulation | -2.32916 | -2.31099 |

In Table S5, we report the energy of the $(H_2)_2$ system of Figure S5 before and after the interaction with the external pulse.

## S3.2 Additional succinic semialdehyde $C_4H_6O_3$ data

In Figure S7, we report selected snapshots of the density displacement (compared to the ground state) in the xy plane following the interaction with the external pulse described in

**Table S5: Energy of the $(H_2)_2$ system of Figure S5 before and after before and after the interaction with the external pulse. Computational details are reported in section S1**

| Energy [a.u.] | Initial | Pulse 1 | Difference [a.u.] |
|---|---|---|---|
| QED simulation: 2 replicas | -4.65989 | -4.62354 | 0.03635 |
| QED simulation: 3 replicas | -6.98988 | -6.93535 | 0.05453 |

section S1 for the succinic semialdehyde $C_4H_6O_3$ in an optical cavity.[1] The figure also shows

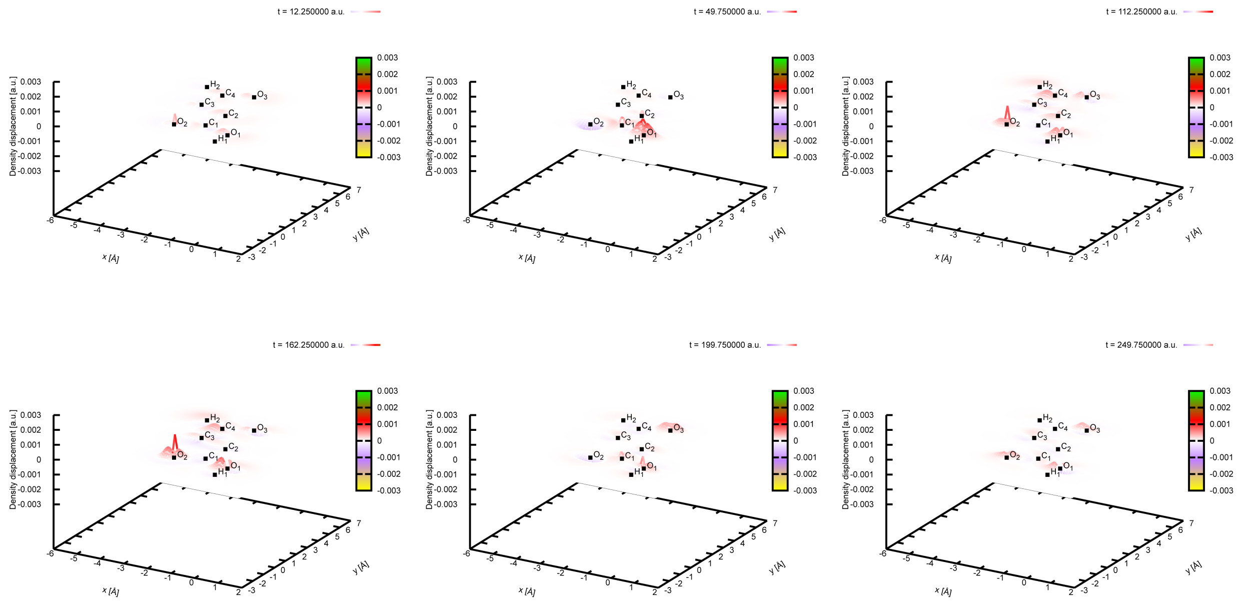


Figure S7: Electronic displacement for the succinic semialdehyde $C_4H_6O_3$ in an optical cavity following the excitation with an external pulse.

the projection of the aldehyde group and the carbon chain on the xy plane (the COO atoms of the acid group lie in the plane while the aldehyde group has small components on z as well, see Table S11). After the pulse has passed, the excitation is mainly localized on the acid group. Compared to the standard (no QED) electronic dynamics, the cavity favors the interaction with the external pulse as more energy is absorbed (see Table S6). As shown in the main text, the electron dynamics is thus fundamentally modified with similar dipole oscillations on x and more intense oscillations on y. The cavity favors a mixing of the states

[1] Videos of the energy-transfer dynamics are available in the following repository: `DOI:10.5281/zenodo.10813660`.

II and III (and partially I), and the two arising middle polaritons have an energy that is closer to the pulse carrier, which favors the interaction with the external pulse.

In Table S6, we report the energy of the succinic semialdehyde $C_4H_6O_3$ of Table S11 before and after the interaction with the external pulse.

**Table S6: Energy of the succinic semialdehyde $C_4H_6O_3$ of Table S11 before and after before and after the interaction with the external pulse. Computational details are reported in section S1**

| Energy [a.u.] | Initial | Pulse 1 | Difference [a.u.] |
|---|---|---|---|
| QED simulation | -380.64662176 | -380.64656622 | 5.554 $10^{-5}$ |
| Reference simulation (no QED) | -380.66605850 | -380.66601210 | 4.640 $10^{-5}$ |

# S4 Real-time QED-CC equations

The RT-QED-CC parametrization for the CC states are

$$|\text{QED-CC}\rangle\,(t) = e^{T(t)}\,|\text{HF},0\rangle\, e^{i\alpha(t)} \tag{3}$$

$$\langle\Lambda|\,(t) = \Bigg(\langle\text{HF},0| + \sum_{(\mu,n)\neq(\text{HF},0)} \bar{t}_{\mu,n}(t)\,\langle\mu,n|\Bigg)e^{-T(t)}e^{-i\alpha(t)}. \tag{4}$$

where, for the QED-CCSD-1 model, the (time-dependent) cluster operator reads

$$T(t) = T_e(t) + T_p(t) + T_{int}(t) \tag{5}$$

$$T_e(t) = \sum_{ai} t_{ai}(t)E_{ai} + \frac{1}{2}\sum_{aibj} t_{aibj}(t)E_{ai}E_{bj} \tag{6}$$

$$T_p(t) = \gamma(t)b^\dagger \tag{7}$$

$$T_{int}(t) = \sum_{ai} s_{ai}(t)E_{ai}b^\dagger + \frac{1}{2}\sum_{aibj} s_{aibj}(t)E_{ai}E_{bj}b^\dagger. \tag{8}$$

The time evolution of these states is determined by the time-dependent Schrödinger equation

$$i\frac{d\,|\text{QED-CC}\rangle}{dt} = H\,|\text{QED-CC}\rangle \tag{9}$$

$$-\,i\frac{d\,\langle\Lambda|}{dt} = \langle\Lambda|\,H. \tag{10}$$

Notice that the parametrization enforces the normalization of the states at all times

$$\langle\Lambda(t)|\text{QED-CC}(t)\rangle = 1. \tag{11}$$

By projection of these equations onto the space $S$ spanned by the zero- and one-photon and singly- and doubly-excited Slater determinants

$$S = \text{Span}\Big\{\,|\text{HF},0\rangle\,, E_{ai}\,|\text{HF},0\rangle\,, E_{ai}E_{bj}\,|\text{HF},0\rangle\,, |\text{HF},1\rangle\,, E_{ai}\,|\text{HF},1\rangle\,, E_{ai}E_{bj}\,|\text{HF},1\rangle\,\Big\} \tag{12}$$

we obtain equations for the time derivatives of the amplitudes, the Lagrange multipliers, and the phase factor[4,5]

$$\frac{d\alpha}{dt} = -\,\langle\text{HF},0|(H+V(t))e^{T(t)}|\text{HF},0\rangle \tag{13}$$

$$\frac{dt_\mu}{dt} = -i\,\langle\mu,0|e^{-T(t)}(H+V(t))e^{T(t)}|\text{HF},0\rangle \tag{14}$$

$$\frac{d\gamma}{dt} = -i\,\langle\text{HF},n|e^{-T(t)}(H+V(t))e^{T(t)}|\text{HF},0\rangle \tag{15}$$

$$\frac{ds_\mu}{dt} = -i\,\langle\mu,n|e^{-T(t)}(H+V(t))e^{T(t)}|\text{HF},0\rangle\,, \tag{16}$$

and

$$\frac{d\bar{t}_{\mu,n}}{dt} = i\,\langle\Lambda|\big[H+V(t),\tau_{\mu,n}\big]\,e^{T(t)}|\text{HF},0\rangle\,, \tag{17}$$

where $\tau_{\mu,n}$ is the excitation operator $\tau_{\mu,n} |\mathrm{HF}, 0\rangle = |\mu, n\rangle$. In response theory, we would resort to a single Fourier component of the external perturbation

$$V_\omega(t) = \left(V^\omega\, e^{-i\omega t} + V^{-\omega} e^{i\omega t}\right) e^{\eta t}, \tag{18}$$

Fourier transforms the equations, and derive an effectively time-independent response equation for the Fourier components of the amplitudes and Lagrange multipliers.[4–7] Once the response functions are obtained, the excitation energies are identified with their poles, and the oscillator strength (and other properties) can be obtained from the residues. In the real-time framework, we propagate the equations from a suitable starting point (usually, the QED-CCSD-1 ground state or the QED-HF state) by using the expression of the time derivatives of the amplitudes. To compute the time derivative, it is sufficient to notice that the expressions correspond to time-dependent $\Omega$ and Jacobian of the QED-CC method.[8,9] A suitable numerical integrator method is thus necessary, such as Runge-Kutta or Euler-Lagrange. The properties in the frequency domain, such as the absorption spectrum, can be obtained from a Fast Fourier Transform of the corresponding time-dependent quantities.[10,11]

# S5 Molecular geometries

In this section, we report the molecular geometries of all the systems studied in the paper.

**Table S7: Molecular geometry of the $(H_2)_2$ system. The coordinates are provided in Angstrom Å.**

| | Atom | x [Å] | y [Å] | z [Å] |
|---|---|---|---|---|
| 1 | H | 0.38 | 0.00 | 0.00 |
| 2 | H | -0.38 | 0.00 | 0.00 |
| 3 | H | 0.50 | 50.0 | 0.00 |
| 4 | H | 0.50 | 50.76 | 0.00 |

**Table S8: Molecular geometry of the $(H_2)_2$ system. The coordinates are provided in Angstrom Å.**

| | Atom | x [Å] | y [Å] | z [Å] |
|---|---|---|---|---|
| 1 | H | 0.38 | 0.00 | 0.00 |
| 2 | H | -0.38 | 0.00 | 0.00 |
| 3 | H | 0.50 | 50.0 | 0.00 |
| 4 | H | 0.50 | 50.78 | 0.00 |

**Table S9: Molecular geometry of the $(H_2)_2$ system. The coordinates are provided in Angstrom Å.**

| | Atom | x [Å] | y [Å] | z [Å] |
|---|---|---|---|---|
| 1 | H | 0.38 | 0.00 | 0.00 |
| 2 | H | -0.38 | 0.00 | 0.00 |
| 3 | H | 0.50 | 5.0 | 0.00 |
| 4 | H | 0.50 | 5.76 | 0.00 |

**Table S10: Molecular geometry of the $(H_2)_2$ system. The coordinates are provided in Angstrom Å.**

| | Atom | x [Å] | y [Å] | z [Å] |
|---|---|---|---|---|
| 1 | H | 0.38 | 0.00 | 0.00 |
| 2 | H | -0.38 | 0.00 | 0.00 |
| 3 | H | 0.50 | 5.0 | 0.00 |
| 4 | H | 0.50 | 5.76 | 0.00 |

**Table S11: Molecular geometry of the succinic semialdehyde $C_4H_6O_3$. The coordinates are provided in Angstrom Å.**

| | Atom | x [Å] | y [Å] | z [Å] |
|---|---|---|---|---|
| 1 | O | 0.000000000000 | 0.000000000000 | 0.000000000000 |
| 2 | O | -2.270583565958 | 0.000000000000 | 0.000000000000 |
| 3 | C | -1.212610304804 | 0.613672647820 | 0.000000000000 |
| 4 | C | -1.068159131583 | 2.120156185050 | 0.011441617514 |
| 5 | C | -2.411117455476 | 2.837430857609 | -0.057315304969 |
| 6 | C | -2.220456659507 | 4.332212528542 | -0.088666176173 |
| 7 | O | -1.119001321111 | 4.871278844754 | -0.047341313890 |
| 8 | H | -0.538724127286 | 2.401902230843 | 0.929108442623 |
| 9 | H | -0.449883807544 | 2.403864608024 | -0.848489638121 |
| 10 | H | -2.961124981613 | 2.547524594807 | -0.958963634409 |
| 11 | H | -3.029742645520 | 2.590464855790 | 0.811921974598 |
| 12 | H | -3.145829269219 | 4.929417388464 | -0.149259067505 |
| 13 | H | -0.085208478076 | -0.977284779926 | -0.002763003539 |

**Table S12: Water molecular geometry. The coordinates are provided in Angstrom Å.**

| | Atom | x [Å] | y [Å] | z [Å] |
|---|---|---|---|---|
| 1 | H | 0.86681 | 0.60144 | 5.00 |
| 2 | H | - 0.86681 | 0.60144 | 5.00 |
| 3 | O | 0.00000 | -0.07579 | 5.00 |

# References


(1) Folkestad, S. D.; Kjønstad, E. F.; Myhre, R. H.; Andersen, J. H.; Balbi, A.; Coriani, S.; Giovannini, T.; Goletto, L.; Haugland, T. S.; Hutcheson, A. et al. e T 1.0: An open source electronic structure program with emphasis on coupled cluster and multilevel methods. *The Journal of Chemical Physics* **2020**, *152*, 184103.

(2) Huber, C.; Klamroth, T. Explicitly time-dependent coupled cluster singles doubles calculations of laser-driven many-electron dynamics. *The Journal of chemical physics* **2011**, *134*.

(3) Feit, M.; Fleck Jr, J.; Steiger, A. Solution of the Schrödinger equation by a spectral method. *Journal of Computational Physics* **1982**, *47*, 412–433.

(4) Koch, H.; Jorgensen, P. Coupled cluster response functions. *The Journal of chemical physics* **1990**, *93*, 3333–3344.

(5) Pedersen, T. B.; Koch, H. Coupled cluster response functions revisited. *The Journal of chemical physics* **1997**, *106*, 8059–8072.

(6) Castagnola, M.; Riso, R. R.; Barlini, A.; Ronca, E.; Koch, H. Polaritonic response theory for exact and approximate wave functions. *Wiley Interdisciplinary Reviews: Computational Molecular Science* **2024**, *14*, e1684.

(7) Olsen, J.; Jørgensen, P. Linear and nonlinear response functions for an exact state and for an MCSCF state. *The Journal of chemical physics* **1985**, *82*, 3235–3264.

(8) Helgaker, T.; Jorgensen, P.; Olsen, J. *Molecular electronic-structure theory*; John Wiley & Sons, 2013.

(9) Haugland, T. S.; Ronca, E.; Kjønstad, E. F.; Rubio, A.; Koch, H. Coupled cluster theory for molecular polaritons: Changing ground and excited states. *Physical Review X* **2020**, *10*, 041043.

(10) Skeidsvoll, A. S.; Balbi, A.; Koch, H. Time-dependent coupled-cluster theory for ultrafast transient-absorption spectroscopy. *Physical Review A* **2020**, *102*, 023115.

(11) Skeidsvoll, A. S.; Moitra, T.; Balbi, A.; Paul, A. C.; Coriani, S.; Koch, H. Simulating weak-field attosecond processes with a Lanczos reduced basis approach to time-dependent equation-of-motion coupled-cluster theory. *Physical Review A* **2022**, *105*, 023103.
